# Supplementary material for: Validity of solid-state Li$^+$ diffusion coefficient estimation by electrochemical approaches for lithium-ion batteries
Source: arXiv:2110.07724 source file (2021-10-14)
Supplement: Supplementary file 1 [file SI.tex]

\newpage
\section*{Supplementary material}

\begin{figure}[!ht]
    \centering
    \includegraphics{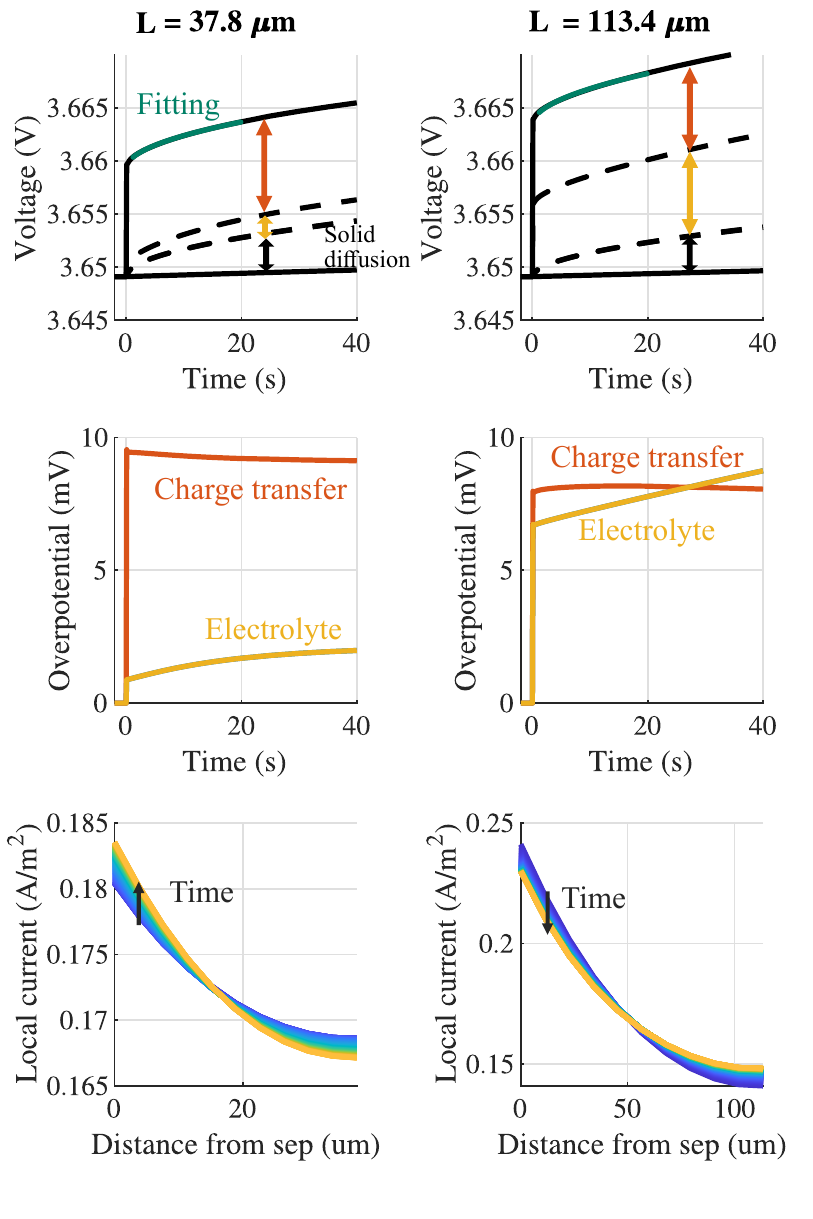}
    \caption{The overpotential and current distribution during a 0.1 C current pulse at $x$ = 0.8. $I$ = 2.49 A/m$^2$ for $L$ = 37.8 $\mu$m, $I$ = 7.47 A/m$^2$ for $L$ = 113.4 $\mu$m.}
    \label{fig:D_s_sweep_current_thickness_analysis}
\end{figure}
